# Supplementary material for: SLADE: Detecting Dynamic Anomalies in Edge Streams without Labels via Self-Supervised Learning
Source: arXiv:2402.11933 source file (2024-07-25)
Supplement: Supplementary file 3 [file 99_appendix_exp.tex]

\begin{table}[t] % command h keeps table in the current position!
    \centering
    \caption{AP (in \%) in the detection of dynamic anomaly nodes. The first method randomly assigns anomaly scores from 0 to 1, and the next four methods are rule-based models, and the others are based on representation learning. 
    For each dataset, the best and the second-best performances are highlighted in \textbf{boldface} and \ul{underlined}, respectively.\label{tab:AP}
    }
    \setlength{\tabcolsep}{2.5pt}
    \small
    \scalebox{1.0}{
        
        \begin{tabular}{l|cccc}
            \toprule
            Method & Wikipedia & Reddit & Bitcoin-alpha & Bitcoin-OTC  \\
            \midrule
            \midrule
                Random Guess & 0.22 $\pm$ 0.05 & 0.09 $\pm$ 0.01 & 8.96 $\pm$ 0.53 & 6.37 $\pm$ 0.28 \\
            \midrule
                \SedanSpot~\citep{eswaran2018sedanspot}  & 0.66 $\pm$ 0.06   & 0.09 $\pm$ 0.00  & 12.99 $\pm$ 0.06        & 16.14 $\pm$ 0.01     \\
                \MIDAS~\citep{bhatia2020midas}  & 0.41 $\pm$ 0.02   & 0.12 $\pm$ 0.00  & 12.99 $\pm$ 0.06        & 16.14 $\pm$ 0.01    \\
                \FFADE~\citep{chang2021f}  & 0.18 $\pm$ 0.00   & 0.09 $\pm$ 0.00  & 6.34 $\pm$ 0.00        & 8.80 $\pm$ 0.00      \\
                \Anoedgel~\citep{bhatia2021sketch}            & 0.18 $\pm$ 0.01   & 0.09 $\pm$ 0.00  & 12.52 $\pm$ 0.86        & 17.03 $\pm$ 0.11    \\
            \midrule 
                \JODIE~\citep{kumar2019predicting} & 1.40 $\pm$ 0.02   & 0.25 $\pm$ 0.05   & 14.31 $\pm$ 0.40  & 15.79 $\pm$ 0.11   \\
                \Dyrep~\citep{trivedi2019dyrep} & 1.53 $\pm$ 0.02   & 0.14 $\pm$ 0.01   & 8.41 $\pm$ 0.58   & 16.14 $\pm$ 1.74   \\
                \TGAT~\citep{xu2020inductive}  & 1.48 $\pm$ 0.14   & 0.27 $\pm$ 0.12   & 12.19 $\pm$ 0.13   & 18.81 $\pm$ 0.63   \\
                \TGN~\citep{tgn_icml_grl2020}  & 1.30 $\pm$ 0.04   & 0.19 $\pm$ 0.01   & 9.65 $\pm$ 0.40   & 19.87 $\pm$ 1.75     \\
                \SAD~\citep{tian2023sad}   & \tb{2.77 $\pm$ 0.91}       & \ul{0.28 $\pm$ 0.06}       & 12.55 $\pm$ 0.58       & 14.33 $\pm$ 0.88 \\
            \midrule
            \rule{0pt}{8pt}
                \tb{\method}
                 & 1.24 $\pm$ 0.14  & 
                 0.23 $\pm$ 0.02  & \tb{15.40 $\pm$ 0.19}  & \ul{20.21 $\pm$ 0.28}   \\
                 \rule{0pt}{10pt}
                \tb{\method-HP}        & \ul{1.56 $\pm$ 0.14}  & \tb{0.30 $\pm$ 0.05}  & \ul{14.86 $\pm$ 0.08}  & \tb{20.46 $\pm$ 0.06} \rule{0pt}{10pt}   \\
            \bottomrule
        \end{tabular}
}
    \normalsize
    % \vspace{-2mm}
\end{table}

%%sedanspot -> 5.5
%MIDAS -> 8.25
%FFADE  -> 9.75
%Anoedge  -> 8.75
%Jodie  -> 4
%Dyrep -> 4.5
%TGAT -> 4.5
%TGN  -> 3.25
%SAD  -> 4.75
%CLADE  -> 1.25
\begin{table}[t!]
    \centering
    \caption{AP (in \%) in the detection of dynamic anomaly nodes in the two synthetic datasets.
    In both datasets, \method performs best compared to unsupervised methods in AP.\label{tab:Email_AP}
    }
    \setlength{\tabcolsep}{2.5pt}
    \small
    \scalebox{1.0}{
        
        \begin{tabular}{l|cc}
            \toprule
            Method & Synthetic-Hijack & Synthetic-New  \\
            \midrule
            \midrule
                Random Guess & 6.61 $\pm$ 0.07 & 6.63 $\pm$ 0.01 \\
            \midrule
                \SedanSpot~\citep{eswaran2018sedanspot}   & 13.95 $\pm$ 1.53   & 15.17 $\pm$ 0.13     \\ \MIDAS~\citep{bhatia2020midas}  & \ul{17.96 $\pm$ 2.56}   & \ul{18.29 $\pm$ 3.18}     \\                \FFADE~\citep{chang2021f}  & 6.57 $\pm$ 0.00   & 6.58 $\pm$ 0.00        \\               \Anoedgel~\citep{bhatia2021sketch}            & 8.20 $\pm$ 0.47   & 8.40 $\pm$ 0.63    \\
            \midrule 
            \rule{0pt}{8pt}
                \tb{\method}
                 &\textbf{69.69 $\pm$ 7.33}  & \textbf{74.46 $\pm$ 6.16} \\
            \bottomrule
        \end{tabular}
}
    \normalsize
\end{table}
\section{Appendix: Additional Experiments}
\label{sec:app:exp}

 \subsection{Performance Evaluation using Average Precision}
\label{sec:app:exp:AP_exp}
In this subsection, we evaluate each model with the Average Precision (AP) metric regarding  RQ1 and RQ4. 
Note that AP has different characteristics from that of the Area Under the ROC Curve (AUC).
While AUC focuses on the overall distinguishability between two different classes, AP focuses on how well a model assigns higher scores for positive samples than for negative samples in terms of precision and recall.
%Thus, for cases where positive samples are rare, including our task (anomaly detection), the AP score is generally lower than the AUC score.}

We utilize the same hyperparameter settings from Section \ref{sec:app:impl:baseline_param} and \ref{sec:app:impl:baseline_param_real}, and include a random guess model that randomly assigns anomaly scores between 0 and 1 for comparison.
As shown in Table~\ref{tab:AP}, \method-HP performs the best or second best in all real-world graph datasets, demonstrating the effectiveness of \method-HP in our task regarding AP also.
Furthermore, as shown in Table~\ref{tab:Email_AP}, \method significantly outperforms other methods in both synthetic datasets.

 \subsection{Variants in Model Architecture}
\label{sec:app:exp:strucutre}
There are two major neural network components in \method: (1) \textbf{GRU}~\citep{chung2014empirical}, which updates the memory of each node, and (2) \textbf{TGAT}~\citep{xu2020inductive}, which generates the memory of a target node.

To demonstrate the effectiveness of each module in dynamic anomaly detection in edge stream, we compare the performances of \method and its several variants where the memory updater and the memory generator are replaced by other neural network architectures.
\begin{comment}
\blue{To demonstrate the effectiveness of each module and explore alternatives, we propose several variants where the memory updater and the memory generator are replaced by other neural network architectures and compare the performance with SLADE.}
\end{comment}

\smallsection{Memory Updater Variant (Instead of GRU)}
\begin{itemize}[leftmargin=*]
    \item \textbf{\method-MLP}: In this variant, we use \textbf{MLP} instead of the GRU module to update the memory of each node.
    Specifically, the memory update procedure (Eq (3) in the main paper) is replaced by the one below:
    \begin{equation}
        \vecs_{i} = \text{MLP}([\vecm_{i} \vert \vert \vecs_{i}]).
    \end{equation}
    Note that in this variant, $\vecm_{i}$ and $\vecs_{i}$ are treated as if they are independent, and thus it cannot capture the temporal dependency between them.
    
    %In this variant, the message and the previous memory are concatenated, and the resulting vector is passed through an MLP to update the memory. 
    %Given this context, memories are generated for each node without considering long-term interaction patterns. The memory update process is as follows: $\vecs_{i}=\text{MLP}([\vecm_{i}||\vecs_{i}])$
    %\item \textbf{CLADE-RNN}: we substitute the GRU with RNN maintaining other structures in this variant. While RNN is capable of capturing some long-term interaction patterns in the memory, when compared to GRU, it encounters the problem of long-term dependencies. The memory update process is as follows: $\vecs_{i}=\text{RNN}(\vecm_{i},\vecs_{i})$      
\end{itemize}

\smallsection{Memory Generator Variants (Instead of TGAT)}
\begin{itemize}[leftmargin=*]
    \item \textbf{\method-GAT}: This variant calculates attention scores based only on the currently given memory information, as follows:
    %While in TGAT, attention is computed by incorporating temporal information, t
    %In this situation, there exists a potential for not effectively capturing short-term interaction patterns. The memory reconstruction process is as follows: 
\begin{align}\label{eq:GAT}
& \hat{\vecs}_{i}=\text{MultiHeadAttention}(\vecq,\textbf{K},\textbf{V}), \ \vecq=\vecs_{i},\\
& \textbf{K}=\textbf{V} = \left [ \vecs_{n_1},...,\vecs_{n_k} \right],  \nonumber
\end{align}
    where $\{n_{1}, ..., n_{k}\}$ denote the indices of the neighbors of the target node $v_i$.
    Note that this variant cannot incorporate temporal information in its attention mechanism.
    \item \textbf{\method-SUM}: In this variant, we use a modified temporal graph sum~\citep{tgn_icml_grl2020} for message passing, as follows:
    %TGAT is replaced with a modified temporal graph sum, as proposed in \citet{tgn_icml_grl2020}, to achieve a simpler and faster aggregation. 
    %Through this approach, temporal information can be taken into account, but attention is not computed for the reconstruction. The memory reconstruction process is as follows: 
\begin{align}\label{eq:sum}
& \hat{\vecs}_{i}=\textbf{W}_{2}(\left [\bar{\vecs}_{i}||\phi(t-t)  \right ]), \nonumber  \\
& \bar{\vecs}_{i}=\text{ReLU}(\sum_{j=1}^{k}\textbf{W}_{1}(\vecs_{n_j}||\phi(t-t'_{n_j}))), \\
& \textbf{W}_{1},\textbf{W}_{2}\in \mathbb{R}^{d_s\times 2d_s},
\nonumber
\end{align}
    where $\{n_{1}, ..., n_{k}\}$ denote the indices of the neighbors of the target node $v_i$, $\{t'_{n_1}, ..., t'_{n_k}\}$ denote the times of the most recent interactions with them, and the weights of each linear layer are denoted as $\textbf{W}_{1}$ and $\textbf{W}_{2}$, respectively.
    Note that this variant does not use any attention mechanism i.e., all neighbors have the same importance.
\end{itemize}
\input{tables/structure_variants}
\begin{figure}[!t]
    % \vspace{-1mm}
    \centering
    \centering
    \includegraphics[width=1\linewidth]{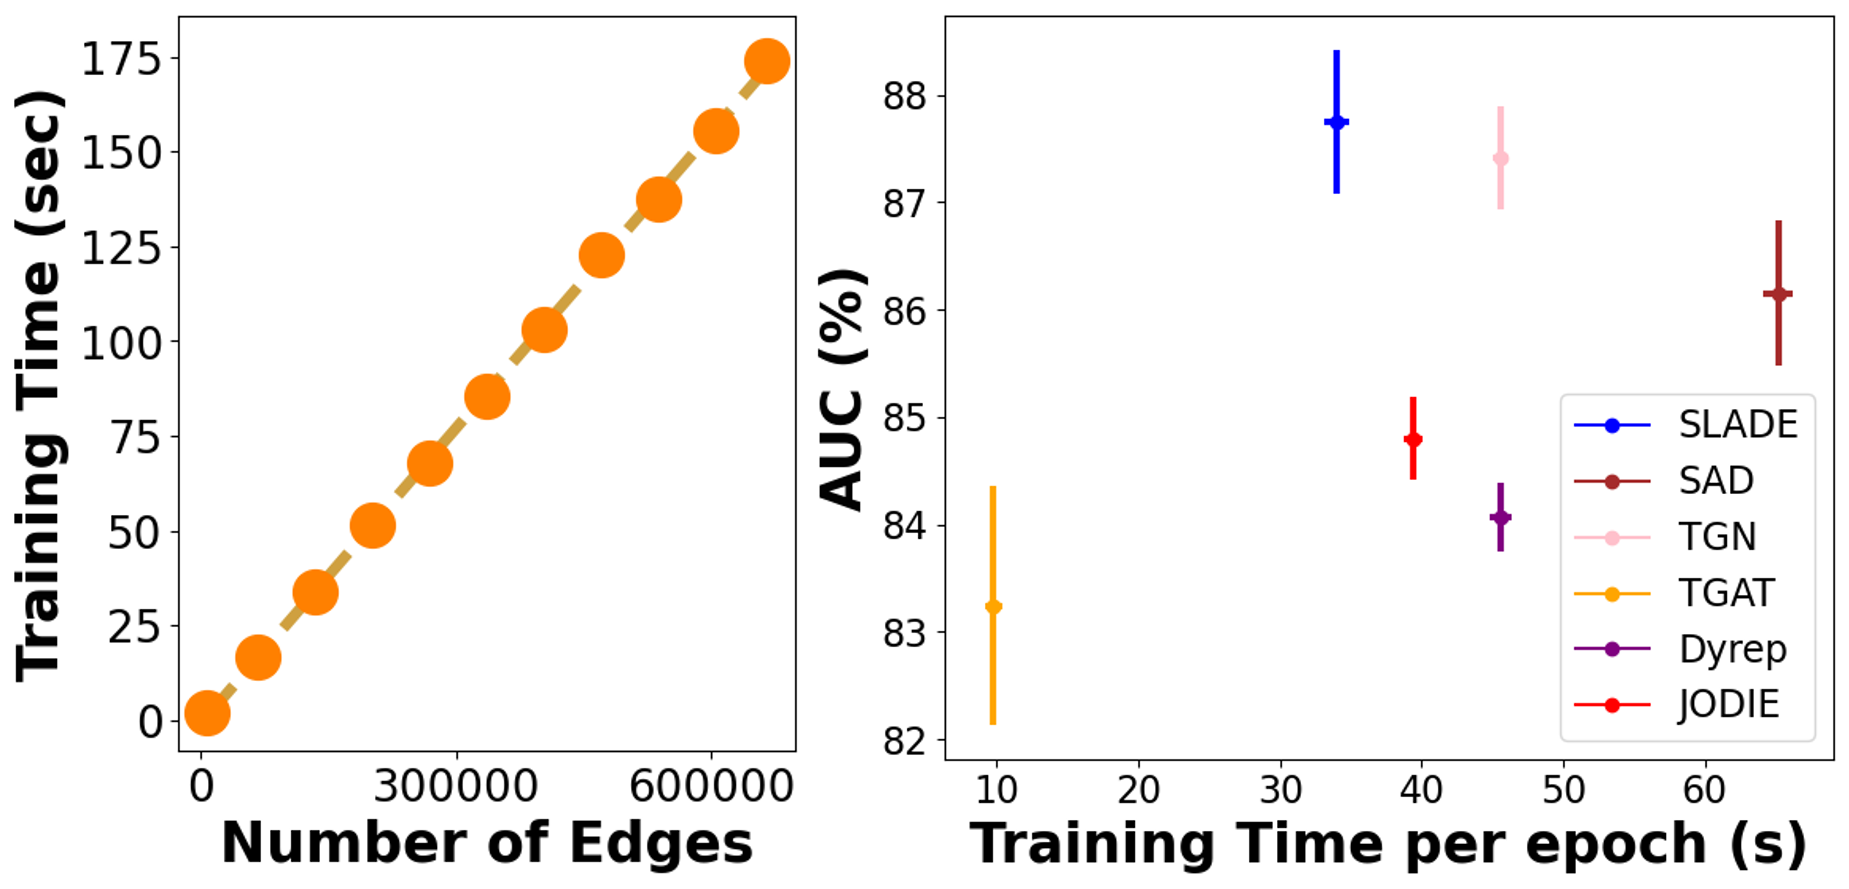} 
    \caption{ \label{fig:trianing_time_analysis}
         The left figure shows the increase in the \blue{training time per epoch} of \method with respect to the number of edges in the Reddit dataset. The right figure shows the training time and AUC score (with standard deviations) in the Wikipedia dataset of the competing learning-based methods.
    }
\end{figure}

\begin{figure*}[t!]
    \begin{subfigure}{0.45\textwidth}
        \centering
        \includegraphics[width=\linewidth]{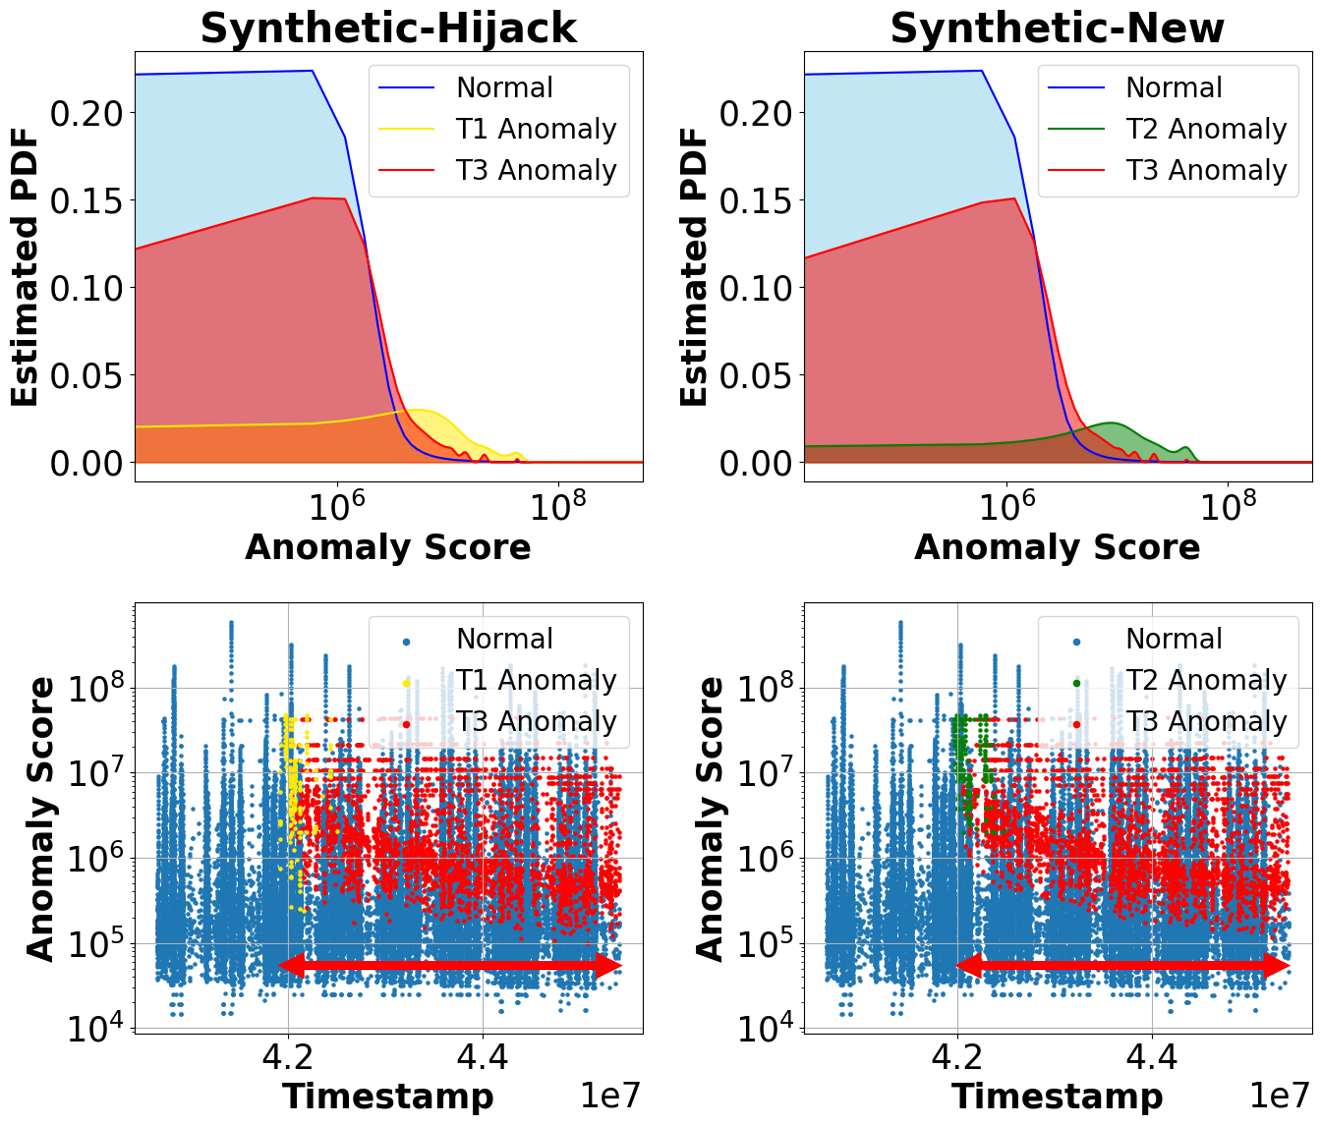}
        \caption*{{(a) Type Analysis of MIDAS}}
        \label{fig:sub1}
        \vspace{0.02\textwidth}
    \end{subfigure}
    \begin{subfigure}{0.45\textwidth}
        \centering
        \includegraphics[width=\linewidth]{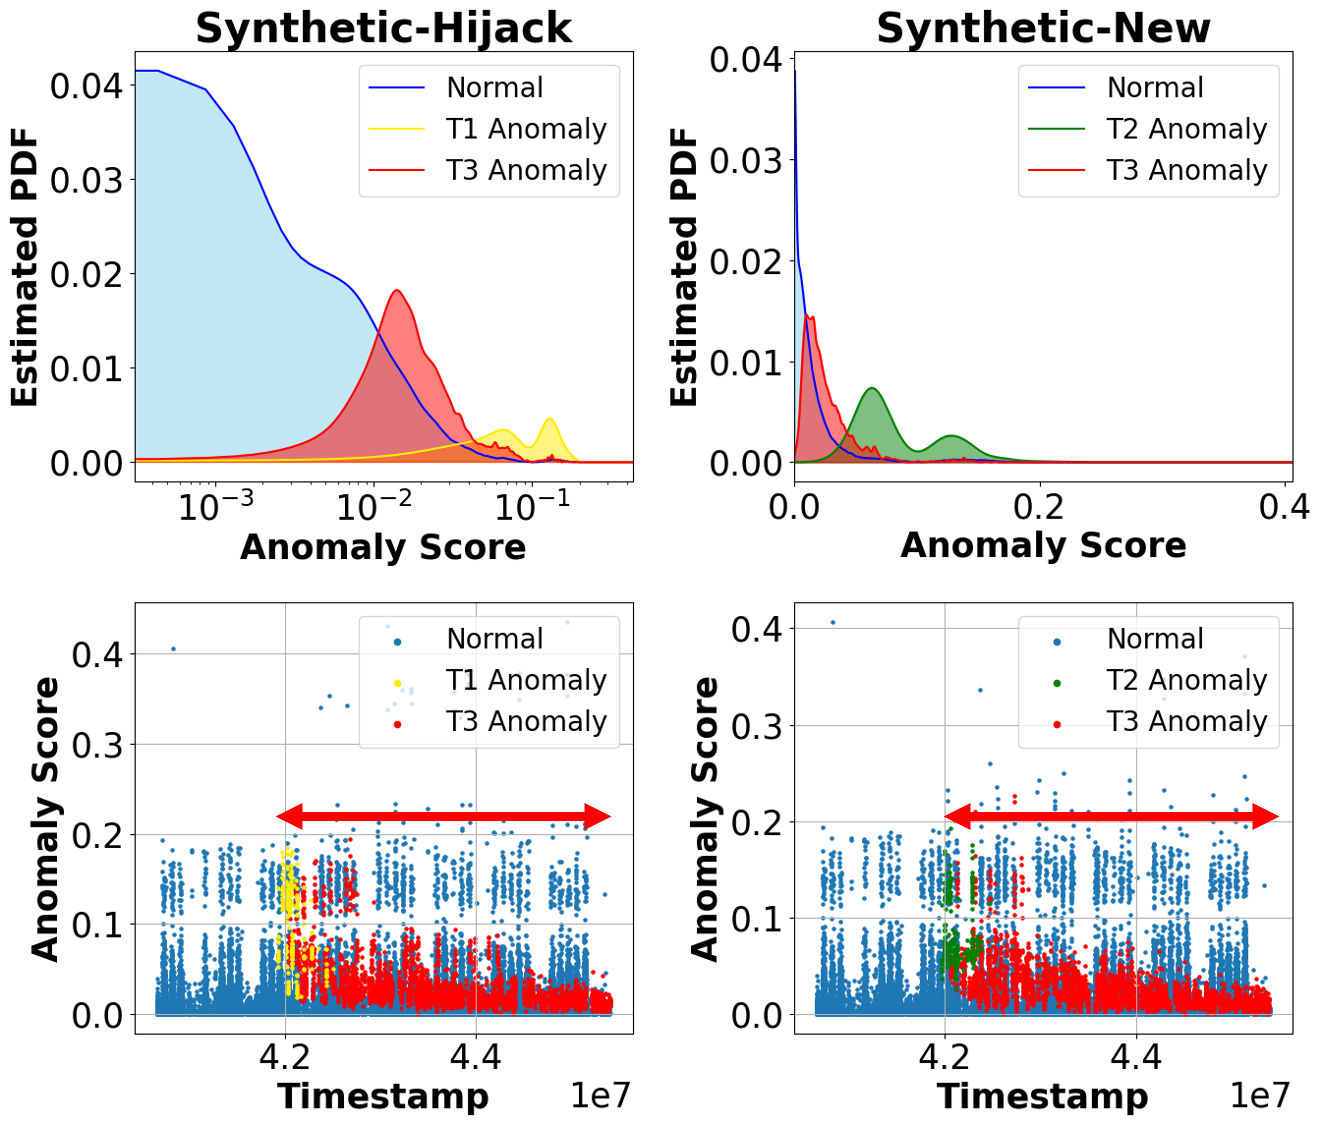}
        \caption*{(b) Type Analysis of SedanSpot}
        \label{fig:sub2}
        \vspace{0.02\textwidth}
    \end{subfigure}
    \caption{ \label{fig:Email_baseline_test}
         For both (a) and (b), the above figures show the distribution of anomaly scores predicted by each baseline for each class in the two synthetic datasets (utilizing kernel density estimation).
         The below figures show the anomaly scores predicted by each baseline over time for each class in both datasets.
         We display the anomaly scores of \MIDAS on a log scale.
    }
\end{figure*}

\smallsection{Experimental Results}
We compare the performances of \method and the introduced three variants, utilizing the same hyperparameter settings as the original \method.
As shown in Table~\ref{tab:variants}, \method achieves the best performance in three out of four datasets.
This result demonstrates the \blue{effectiveness} of GRU and TGAT, i.e., the importance of modeling temporal dependency in memory updating and temporal attention in memory generation.
%Hyperparameter setting of \method variants is fixed as that of the original \method.
%\footnote{Hyperparameters of variants models are fixed as the original \method setting.}.
Specifically, \method-MLP and \method-GAT consistently underperform \method and \method-SUM, demonstrating the importance of utilizing temporal information and temporal dependency in detecting dynamic anomalies.
%\blue{
%In contrast, SLADE-SUM can be considered a quite effective variant, outperforming other baselines across most datasets.
%However, Incorporating temporal attention through TGAT further enhances performance.
%}
Furthermore, while \method-SUM outperforms \method in the Wikipedia dataset, its performance gain is marginal (within the standard deviation).

\subsection{Model Training Speed}\label{sec:app:exp:training}
In this subsection, we analyze the training time of \method.

We first empirically demonstrate the training time of \method on the Reddit dataset with varying edge counts, where the detailed setting is the same as that described in Section 6.2 of the main paper.
As shown in the left plot of Figure~\ref{fig:trianing_time_analysis}, the training runtime of \method is almost linear in the number of edges.
Since the number of edges is much greater than that of nodes ($67\times$), the overall scale is dominated by the number of edges.

Furthermore, we compare the empirical training time of \method against that of other neural network-based methods, which require the training procedure.
As shown in the right plot of Figure~\ref{fig:trianing_time_analysis}, in terms of the empirical training speed, \method is competitive compared to other methods.
Specifically, among six neural network-based dynamic anomaly detection methods, \method exhibits the second-fastest training time, showing the best anomaly detection performance.

\subsection{Type Analysis of Baselines}
\label{sec:app:exp:scenario}

We conduct an additional analysis regarding two baseline methods (\MIDAS and \SedanSpot), which ranked second- and third-best position in our synthetic data experiments (\textbf{RQ4}).
First, as shown in the first row of Figure~\ref{fig:Email_baseline_test} (a) and (b), we verify that the score distribution of the normal class and that of the consistent anomaly class ({\textbf{T3}}) largely overlaps in both models.
Moreover, as shown in the second row of Figure~\ref{fig:Email_baseline_test}(a) and (b), \MIDAS and \SedanSpot assign relatively high scores when anomalies of \textbf{T1} and \textbf{T2} occur, but not as distinctly as \method.
These two results indicate that previous unsupervised anomaly detection baselines fail to detect anomalies if anomalies do not align with the targeted anomaly pattern, leading to high false negatives.
These results emphasize the necessity of learning-based unsupervised anomaly detection models (\method), which autonomously learn normal patterns, and are capable of detecting a wide range of anomalies by finding cases that deviate from the learned normal patterns.

\blue{
%\section{Additional Experimental Results}
%\label{sec:app:dataset}
\subsection{Self-supervised Task with Edge Prediction}
\label{sec:app:SSL_edge}
In this subsection, we evaluate the performance of the link prediction-based self-supervised task (We denominate this task as S3). We train each neural network baseline method based on S3 and use the negative prediction probability score of the target node's involved edge as its anomaly score without fine-tuning a classifier with labels. 
In this case, anomaly detection can be performed based on the unexpectedness of the interaction in which the target node is involved.
As shown in Table~\ref{tab:Edge_SSL_auc}, S3 is less effective in performing dynamic anomaly detection compared to our proposed node-wise self-supervised tasks (S1, S2). 
In predicting the dynamic states of nodes, we expect that the edge-wise self-supervised task has weaker expressive power to distinguish dynamic states compared to node-wise self-supervised tasks.
For example, if two users from different departments exchange an email in the email network, the unexpectedness of the interaction might be greater than the unexpectedness of an interaction performed by an anomalous user who randomly sends spam emails to various users.
}

\blue{
Our additional edge frequency analysis in Fig~\ref{fig:Edge_SSL_analysis} supports this claim. 
If the edges that the anomalous state nodes are involved in are indeed unexpected, we can expect edges with the same node pair composition as those involving anomalous nodes to occur much less frequently compared to other normal edges in the dataset. 
However, upon comparing the frequency distributions of normal edges and anomalous edges, 
we observe no clear distinction between the two distributions in Wikipedia and Reddit datasets.} %when detecting dynamic anomalies in edge streams.

\begin{table}[h!]
    \centering
    \caption{\label{tab:Edge_SSL_auc} AUC (in \%) in the detection of dynamic anomaly nodes with baselines based on link prediction self-supervised task.}
    \setlength{\tabcolsep}{2.5pt}
    \small
    \scalebox{1.0}{
        
        \begin{tabular}{l|cc}
            \toprule
            Method & Wikipedia & Reddit  \\
            \midrule
            \midrule
                \JODIE (S3)~{\citep{kumar2019predicting}} & 68.88 $\pm$ 1.54   & 58.17 $\pm$ 0.55     \\
                \Dyrep (S3)~{\citep{trivedi2019dyrep}} & 58.78 $\pm$ 4.79   & 59.61 $\pm$ 1.22     \\
                \TGAT (S3)~{\citep{xu2020inductive}}  & 71.40 $\pm$ 2.25   & 59.86 $\pm$ 1.48      \\
                \TGN (S3)~{\citep{tgn_icml_grl2020}}  & 58.05 $\pm$ 3.48   & 56.77 $\pm$ 0.13       \\
            \midrule
            \rule{0pt}{8pt}
                \tb{\method} (S1,S2)
                 &\bf{87.75 $\pm$ 0.68}  & \bf{72.19 $\pm$ 0.60}    \\
            \bottomrule
        \end{tabular}
}
\end{table}
%\vspace{-1cm}
\begin{figure}[H]
    \centering
    \setlength\aboverulesep{0.5pt}
    \setlength\belowrulesep{0.5pt}
    \centering
    \includegraphics[width=1\linewidth]{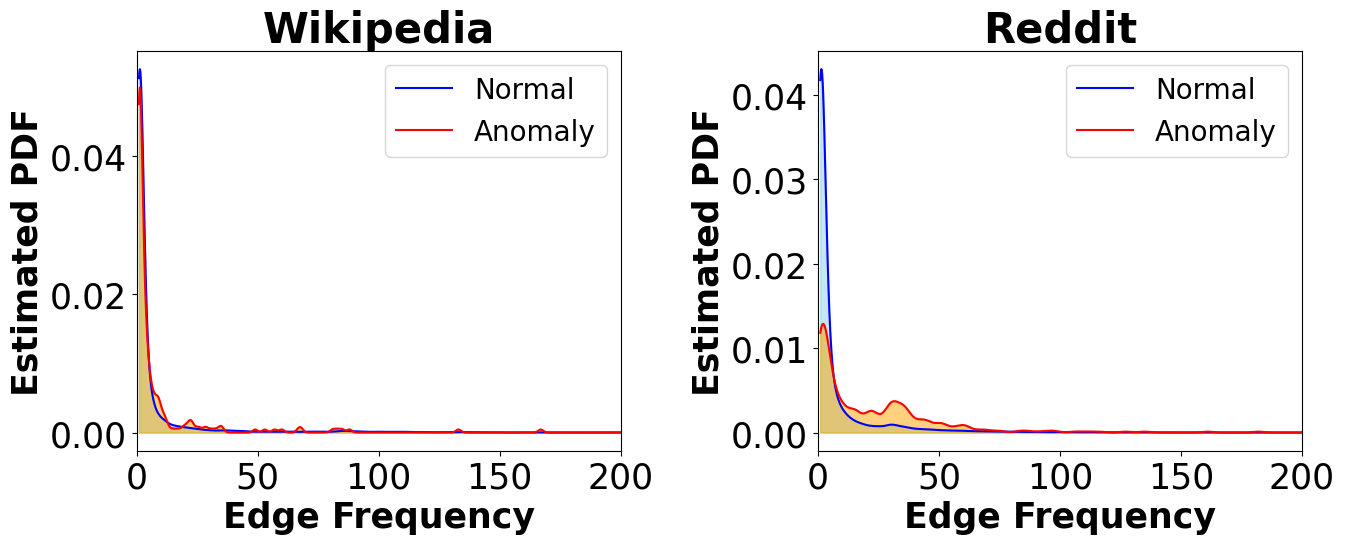} 
    \caption{
    \label{fig:Edge_SSL_analysis} The above figures show the frequency distribution of edges with the same node pair composition as those involving anomalous nodes compared to normal edges in Wikipedia and Reddit datasets. 
    }
\end{figure}

\blue{
\subsection{DTDG and Static Graph-based baselines}
In this subsection, We evaluate the dynamic anomaly detection performance of DTDG and static graph-based anomaly detection methods using real-world datasets. We utilize two SOTA DTDG-based approaches, StrGNN and TADDY, and one static graph-based approach, DOMINANT. The experimental setting is the same as that of our Section 6.2 RQ1 experiment. 
We follow the hyperparameter settings provided by the existing DTDG papers with the exception of the number of epochs, which is reduced to 10 due to the long training time of DTDG methods.
Regarding DOMINANT, as there is no node feature in our datasets, we utilize identity vectors as node features.  
According to Table~\ref{tab:DTDG_static}, SLADE outperforms other baselines. We expect that DTDG-based methods primarily aim for anomalous edge detection, which is less effective for node-wise dynamic anomaly detections, as mentioned in Section~\ref{sec:app:SSL_edge}.
Additionally, static graph-based baselines like Dominant will struggle to predict dynamically changing states, as they cannot leverage temporal information.}

\begin{table}[H]
    \centering
    \caption{\label{tab:DTDG_static} AUC (in \%) in the detection of dynamic anomaly nodes with DTDG-based baselines and a static graph-based baseline.}
    \setlength{\tabcolsep}{2.5pt}
    \small
    \scalebox{0.95}{
        
        \begin{tabular}{l|cccc}
            \toprule
            Method & Wikipedia & Reddit & Bitcoin-alpha & Bitcoin-OTC  \\
            \midrule
            \midrule
                DOMINANT~{\citep{ding2019deep}} & 67.15 $\pm$ 1.38   & 44.17 $\pm$ 0.53   & 54.21 $\pm$ 8.78  & 51.26 $\pm$ 0.01   \\
                STrGNN~{\citep{cai2021structural}} & 50.95 $\pm$ 0.46   & 53.30 $\pm$ 0.22   & 51.26 $\pm$ 0.01  & 47.85 $\pm$ 0.15   \\
                TADDY~{\citep{liu2021anomaly}} & 56.48 $\pm$ 1.41   & 54.54 $\pm$ 0.43   & 57.52 $\pm$ 1.41   & 64.06 $\pm$ 0.38    \\
            \midrule
            \rule{0pt}{8pt}
                \tb{\method}
                 &\bf{87.75 $\pm$ 0.68}  & \bf{72.19 $\pm$ 0.60}  & \bf{76.32 $\pm$ 0.28}  & \bf{75.80 $\pm$ 0.19}   \\
            \bottomrule
        \end{tabular}
}
    \vspace{-2.5mm}
\end{table}
\blue{
\subsection{Robustness to Anomalies in Training}
In this subsection, we assess SLADE's robustness to anomalies within the training set with the baseline (SAD).
We augment the training dataset with increasing known abnormal edges, which are the edges involving nodes with the anomalous state in the training set, equivalent to X\% of the training dataset size, denoted as dataset+X\%.
These anomalies are assumed to remain undetected and are considered normal during the training phase.
%The anomaly ratio in the Wikipedia test set is 0.186\%, while it is 0.09\% in the Reddit test set.
As shown in Table~\ref{tab:robust}, while the performance drop of SLADE is at most 0.023 AUROC, that of the baseline method is at most 0.691 AUROC. 
SLADE demonstrates good performance even when abnormal data within the training dataset is significant (over 10\% of total edge), showing its robustness.}

\begin{table}[H]
    \centering
    \caption{\label{tab:robust} AUC (in \%) in the detection of dynamic anomaly nodes against additional anomalies in the training set.}
    \setlength{\tabcolsep}{2.5pt}
    \small
    \scalebox{1.0}{
        
        \begin{tabular}{l|cc}
            \toprule
            Dataset & SLADE & SAD~{\citep{tian2023sad}}   \\
            \midrule
            \midrule
                WIKI+0
                \% & 87.75 $\pm$ 0.68   & 86.15 $\pm$ 0.63     \\
                WIKI+1
                \% & 87.48 $\pm$ 0.56   & 62.64 $\pm$ 13.55     \\
                WIKI+10
                \%  & 87.33 $\pm$ 0.59   & 17.04 $\pm$ 15.77    \\
                WIKI+20
                \%  & 87.05 $\pm$ 3.48   & 33.76 $\pm$ 6.86       \\
            \midrule
                REDDIT+0
                \% & 72.19 $\pm$ 0.60   & 68.45 $\pm$ 1.27     \\
                REDDIT+1
                \% & 72.10 $\pm$ 0.47   & 51.18 $\pm$ 1.28     \\
                REDDIT+10
                \%  & 71.69 $\pm$ 0.92   & 46.64 $\pm$ 0.95    \\
                REDDIT+20
                \%  & 69.97 $\pm$ 4.50   & 47.07 $\pm$ 1.51       \\
            \bottomrule
        \end{tabular}
}
\end{table}

\blue{
\subsection{SLADE with Label Supervision}
In this subsection, we evaluate the variants of SLADE utilizing the proposed self-supervised tasks (S1, S2) as pretext tasks and then fine-tuning models with labels.
Specifically, models in SLADE are first pre-trained with our proposed self-supervised tasks (S1, S2), and then dynamic representations (current memory, previous memory, generated memory) from SLADE and label information are utilized to fine-tune the MLP decoder. 
In the zero-shot setting, only normal labels are utilized. 
We denote SLADE-FT as SLADE with a fine-tuning and SLADE-ZS as SLADE with a zero-shot setting.
We conduct experiments with the same settings with SLADE on the proposed real-world datasets. 
As shown in Table~\ref{tab:fine_tuning}, surprisingly, our finding is that utilizing additional fine-tuning with label information is less effective than our method in most cases. 
We expect that our self-supervised tasks (S1, S2) already align well with dynamic anomaly detection, while minimal anomaly label supervision may introduce issues such as distribution shift.
}

\begin{table}[H]
    \centering
    \caption{\label{tab:fine_tuning} AUC (in \%) in the detection of dynamic anomaly nodes with fine-tuning variant (SLADE-FT) and zero-shot variant (SLADE-ZS) of SLADE.}
    \setlength{\tabcolsep}{2.5pt}
    \small
    \scalebox{1.0}{
        
        \begin{tabular}{l|cccc}
            \toprule
            Method & Wikipedia & Reddit & Bitcoin-alpha & Bitcoin-OTC  \\
            \midrule
            \midrule
                SLADE-FT & 86.06 $\pm$ 0.14   & 60.04 $\pm$ 0.55   & \bf{77.08 $\pm$ 0.17}  & 73.14 $\pm$ 0.61   \\
                SLADE-ZS & 59.15 $\pm$ 0.09   & 53.34 $\pm$ 3.05   & 72.69 $\pm$ 0.02   & 65.00 $\pm$ 0.43    \\
            \midrule
            \rule{0pt}{8pt}
                \tb{\method}
                 &\bf{87.75 $\pm$ 0.68}  & \bf{72.19 $\pm$ 0.60}  & 76.32 $\pm$ 0.28  & \bf{75.80 $\pm$ 0.19}   \\
            \bottomrule
        \end{tabular}
}
    \vspace{-2.5mm}
\end{table}
\blue{
\subsection{SLADE in Large-scale Scenarios}
We create a large-scale synthetic dataset using TGBL-coin dataset from the Temporal Graph Benchmark~\citep{huang2024temporal} Dataset. 
In TGBL-coin dataset, each node is an address, and each temporal edge is the transaction of funds from one node to another with time information.
We reduce the dataset size (due to time constraints in the experiment) and preprocess the dataset by utilizing the same anomaly injection method in Section 6.2 RQ4, and it contains 499K nodes and 11M edges with a 1\% anomaly ratio.
Due to the significant resource and time requirements for training on such a large-scale dataset, we utilize only 30\% of the data for training and the remaining 70\% for testing.
We employ rule-based methods for baselines and follow the same setting with RQ4 testing. 
We utilize almost the same hyperparameters in SLADE, modifying the training epoch to 3 due to training cost and overfitting.
Our experimental result in Table~\ref{tab:large} demonstrates that SLADE also performs well on large-scale datasets compared to other baselines. 
}

\blue{
Additionally, we empirically analyze the scalability of SLADE's training and inference processes in large-scale scenarios by applying the same approach as in Section 6 RQ2 and Appendix~\ref{sec:app:exp:training} to tgbl-coin. 
Regarding inference time, we observe that SLADE maintains a constant inference time per edge, even on large-scale datasets.
This reaffirms that SLADE has an inference time complexity independent of graph size, as mentioned in Section 6 RQ2. 
On the other hand, unlike in Appendix~\ref{sec:app:exp:training}, we observe that the training time increases more than linearly with the number of edges in a large-scale dataset.
As roughly analyzed in Appendix E.2, this increase is likely due to the large number of nodes appearing in the training set for negative sampling, which impacts the training time.
%Therefore, SLADE has room for improvement in terms of training complexity in large-scale scenarios. 
%To address this issue, we need to devise strategies such as limiting the number of negative samples.
}

\begin{table}[H]
    \centering
    \caption{\label{tab:large} AUC (in \%) in the detection of dynamic anomaly nodes with unsupervised baselines in the TGBL-coin dataset.}
    \setlength{\tabcolsep}{2.5pt}
    \small
    \scalebox{1.0}{
        
        \begin{tabular}{l|c}
            \toprule
            Method & TGBL-coin   \\
            \midrule
            \midrule
                \MIDAS~{\citep{bhatia2020midas}} & 56.16 $\pm$ 0.58     \\
                SedanSpot~{\citep{eswaran2018sedanspot}} & 77.14 $\pm$ 0.22  \\
                F-FADE~{\citep{chang2021f}}  & 59.33 $\pm$ 0.00  \\
                Anoedge-l~{\citep{cormode2005improved}}  & 39.11 $\pm$ 2.72  \\
            \midrule
            \rule{0pt}{8pt}
                \tb{\method} 
                 &\bf{83.17 $\pm$ 1.34} \\
            \bottomrule
        \end{tabular}
}
    \vspace{-2.5mm}
\end{table}
\begin{figure}[H]
    \centering
    \setlength\aboverulesep{0.5pt}
    \setlength\belowrulesep{0.5pt}
    \centering
    \includegraphics[width=1\linewidth]{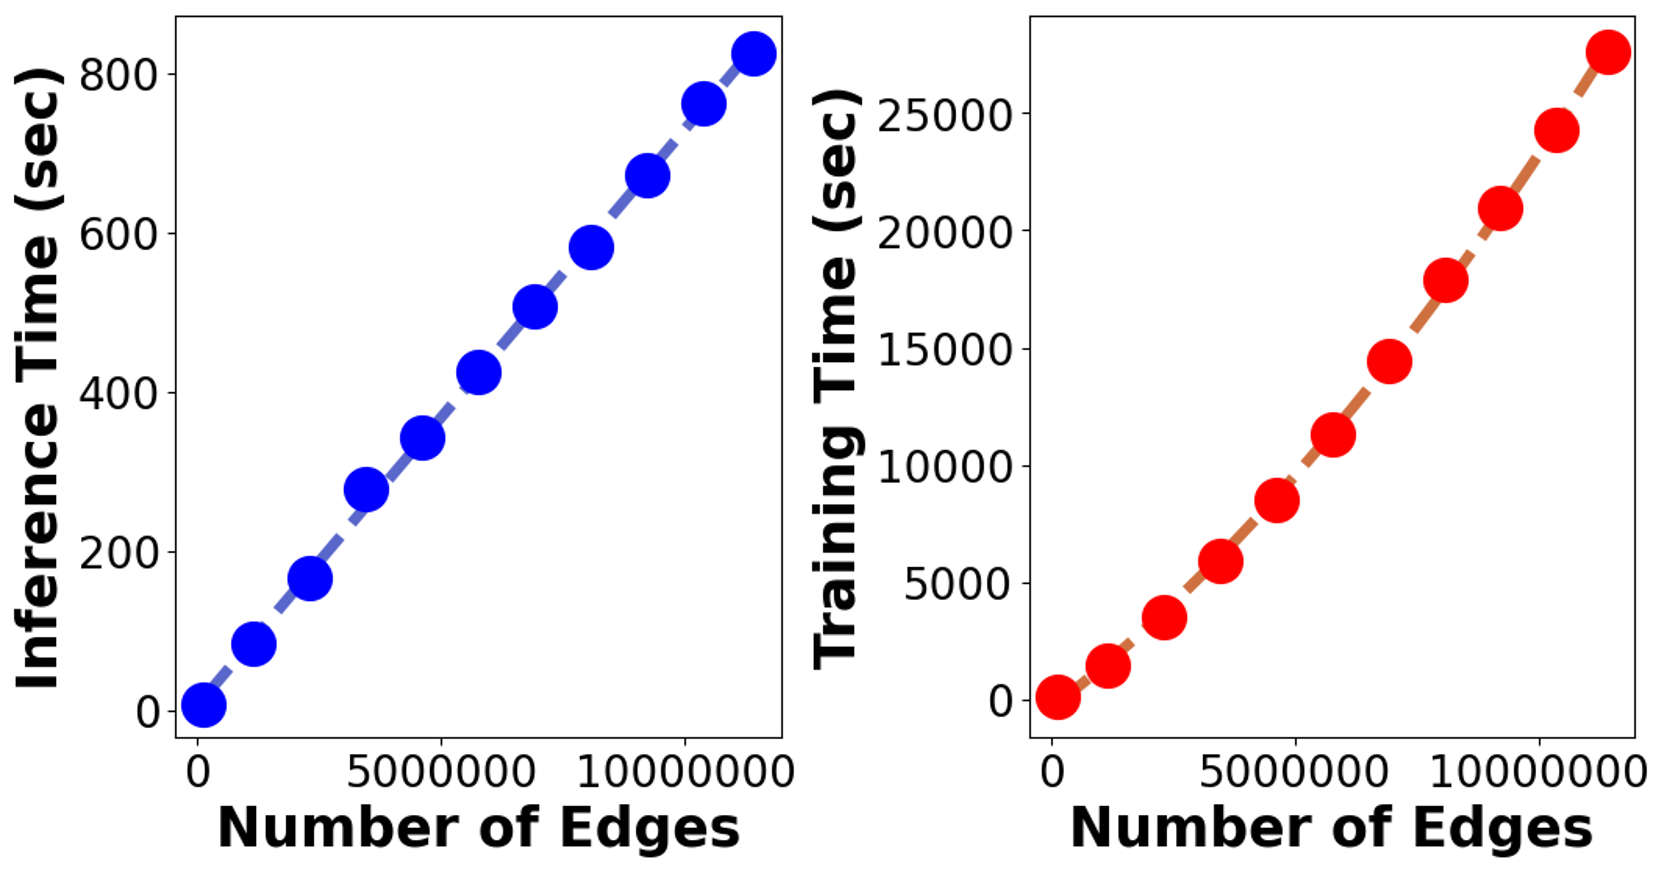} 
    \caption{
    \label{fig:Transportation} The left figure shows the increase in the inference time and the right figure shows the increase in the training time per epoch of \method with respect to the number of edges in a large-scale scenario. 
    }
\end{figure}

\blue{
\subsection{Learnable Time Encoding}
In this subsection, we evaluate the performance difference based on whether the time encoding is trained using the TGAT~\citep{xu2020inductive} approach or fixed using the GraphMixer~\citep{cong2022we} approach.
SLADE utilizes time encodings with fixed weights, as suggested by GraphMixer. We construct a variant of our model that utilizes learnable time encoding (SLADE-LT) from TGAT and compare it with SLADE with fixed time coding (SLADE-FT). According to Table~\ref{tab:TE}, we empirically verify that SLADE-FT encoding performs better. 
We hypothesize that this is due to the distribution shift issue. 
First, our dynamic node anomaly detection task can be considered as a (temporal) extrapolation task.
Thus, test data may follow a different time-interval distribution from that of training data.
Consequently, learnable time encoding, which is likely to overfit the train data, may exhibit poor generalization to the test data, leading to suboptimal dynamic anomaly detection performance.}

\begin{table}[H]
    \centering
    \caption{\label{tab:TE} AUC (in \%) in the detection of dynamic anomaly nodes with a learnable time encoding variant (SLADE-LT) of SLADE and SLADE (SLADE-FT). }
    \setlength{\tabcolsep}{2.5pt}
    \small
    \scalebox{1.0}{
        
        \begin{tabular}{l|cccc}
            \toprule
            Method & Wikipedia & Reddit & Bitcoin-alpha & Bitcoin-OTC  \\
            \midrule
            \midrule
                SLADE-LT & 86.78 $\pm$ 0.66   & 65.28 $\pm$ 0.68   & 71.11 $\pm$ 0.83  & 73.98 $\pm$ 0.35   \\
                \tb{\method-FT}
                 &\bf{87.75 $\pm$ 0.68}  & \bf{72.19 $\pm$ 0.60}  & 76.32 $\pm$ 0.28  & \bf{75.80 $\pm$ 0.19}   \\
            \bottomrule
        \end{tabular}
}
    \vspace{-2.5mm}
\end{table}

\blue{
\subsection{Transportation Network Dataset}}
\blue{We evaluate the performance of SLADE in a transportation network, which belongs to a different domain than the datasets used in the main experiments.
We utilize the New York  (NYC) Taxi dataset (Yellow Taxi Trip Records from TLC Record data~\footnote{https://www.nyc.gov/site/tlc/about/tlc-trip-record-data.page} in December 2023) and split the data into training and test sets chronologically, with each set comprising 50\% of the data.
In the transportation network, each node represents a NYC taxi zone location. We preprocess temporal edges to represent NYC taxi trips, with the source node as the departure taxi zone, the destination node as the arrival taxi zone, and the time as the arrival time.
Since the dataset does not contain labels indicating anomalies, we aim to analyze the trend between the daily average anomaly scores of NYC taxi trips and actual events that occurred.
As shown in Figure~\ref{fig:Transportation}, SLADE assigns higher anomaly scores for 12/25 (Christmas) and 12/31 (the last day of the year), which exhibit different transportation patterns than other days. 
}
\begin{figure}[H]
    \centering
    \setlength\aboverulesep{0.5pt}
    \setlength\belowrulesep{0.5pt}
    \centering
    \includegraphics[width=1\linewidth]{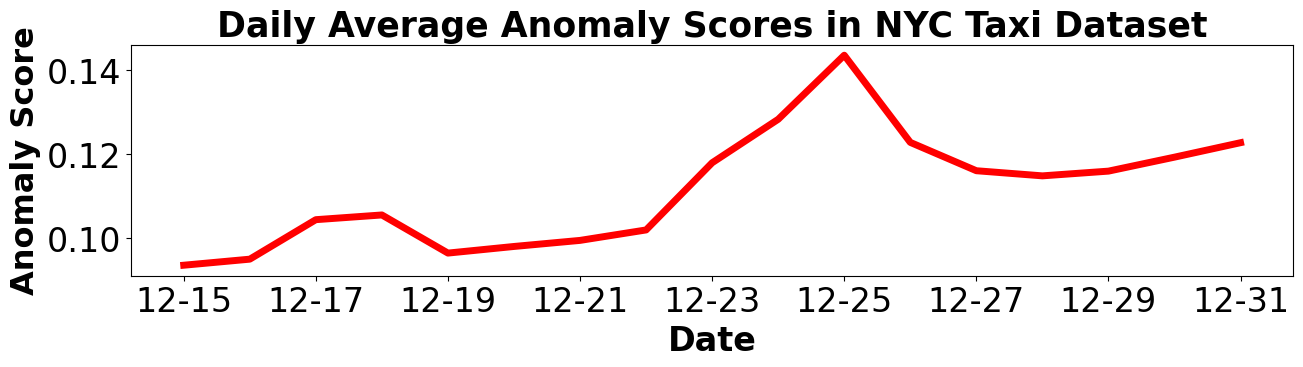} 
    \caption{
    \label{fig:Transportation} Daily average anomaly scores of NYC taxi trips in December 2023. 
    }
\end{figure}

\blue{
\subsection{Anomalies with Camouflage}}
\blue{
In this subsection, we assess the robustness of SLADE in dealing with camouflaging attackers who alternate between anomalous and normal behaviors.
To reflect this case, we conduct a dynamic anomaly detection task on our new synthetic dataset: Synthetic-Hide, where camouflaged anomalous nodes exist.
Specifically, unlike Synthetic-Hijack, we first select anomalous node candidates from only normal nodes that continuously appear in the test set.
Subsequently, we follow the same previous anomaly injection method with the same 1\% anomaly injection in Appendix~\ref{sec:app:dataset}. Through this method, anomalous nodes are considered to perform normal interactions with similar neighbors for hiding and anomalous interactions with random neighbors for attack. 
We evaluate the performance of SLADE on Synthetic-Hide against unsupervised baselines using the same settings in Appendix~\ref{sec:app:base:baseline_real}.
As shown in Table~\ref{tab:Email_hide}, SLADE still outperforms other competing unsupervised methods by a significant gap. 
However, compared to the case without camouflaged actions (Synthetic-New dataset), we demonstrate a slight decrease in the SLADE's performance.
}

\blue{
In the situation where an attacker consistently engages in abnormal interactions that mimic our proposed normal patterns (A1, A2), there is indeed a possibility of deceiving SLADE.
Nonetheless, as discussed in Section 4, such scenarios require the attacker to consistently engage in these abnormal interactions with similar targets (i.e., victims) over an extended period. 
These repeated interactions impose significant costs on attackers. Moreover, targeting similar victims repeatedly may increase the likelihood of detection, such as through reports from the victims.
As a result, anomalous nodes are likely to exhibit interaction patterns opposite to our proposed normal patterns.
%However, if an attacker consistently engages in abnormal interactions that mimic our proposed normal patterns (A1, A2), there is indeed a possibility of deceiving SLADE.
%Nonetheless, as discussed in Section 4, such scenarios would require the attacker to consistently engage in these abnormal interactions with similar targets (i.e., victims) over an extended period. 
%These repeated interactions impose significant costs on attackers. Moreover, targeting similar victims repeatedly may increase the likelihood of detection, such as through reports from the victims.
%As a result, anomalous nodes are likely to exhibit interaction patterns opposite to our proposed normal patterns.
}

\begin{table}[H]
    \centering
    \caption{AUC (in \%) in the detection of dynamic anomaly nodes in Synthetic-Hide and Synthetic-New.
    In both datasets, \method performs best compared to unsupervised methods in AUC.\label{tab:Email_hide}
    }
    \setlength{\tabcolsep}{2.5pt}
    \small
    \scalebox{1.0}{
        
        \begin{tabular}{l|cc}
            \toprule
            Method & Synthetic-Hide & Synthetic-New  \\
            \midrule
            \midrule                \SedanSpot~\citep{eswaran2018sedanspot}   & 75.18 $\pm$ 2.12   & 78.05 $\pm$ 1.68     \\ \MIDAS~\citep{bhatia2020midas}  & \ul{81.78 $\pm$ 0.09}   & \ul{82.63 $\pm$ 0.07}     \\                \FFADE~\citep{chang2021f}  & 41.54 $\pm$ 0.00   & 48.73 $\pm$ 0.00        \\               \Anoedgel~\citep{bhatia2021sketch}            & 60.57 $\pm$ 2.11   & 61.86 $\pm$ 2.41    \\
            \midrule 
            \rule{0pt}{8pt}
                \tb{\method}
                 &\textbf{96.11 $\pm$ 3.31}  & \textbf{98.38 $\pm$ 1.09} \\
            \bottomrule
        \end{tabular}
}
    \normalsize
\end{table}

\blue{
\subsection{Dynamic Heterogeneous Graphs}}
\blue{
SLADE performs anomaly detection on dynamic homogeneous graphs in the main experiments.
However, nodes and edges in specific real-world networks can have different types, forming dynamic heterogeneous graphs.
In this case, SLADE can assume that the same type exhibits similar normal interaction patterns (A1, A2), and specific normal interaction patterns vary depending on the types.
Thus, we can perform anomaly detection on dynamic heterogeneous graphs for each type separately by creating distinct memory updater and generator models as in SLADE.
Despite this, we encounter challenges due to the absence of suitable datasets and baselines for anomaly detection in dynamic heterogeneous graphs.
Recently, \citep{li2023thgnn} has proposed a DTDG-based approach for anomalous edge detection and provided related datasets, but we have not found any datasets specifically tailored for anomalous node detection in edge streams.
%We anticipate that further research will be needed in this area.
}

\blue{
Although they cannot replace dynamic heterogeneous graphs, we can consider bipartite graphs as a kind of simple dynamic heterogeneous graph with two types of nodes. Among our datasets, Wikipedia and Reddit are bipartite graphs between users and items.
We design SLADE-Hetero for a dynamic bipartite graph by utilizing different memory updaters and generators for each node type to train distinct normal patterns of each type.
Then, we compare SLADE-Hetero with the original SLADE, and most of its settings are identical to SLADE described in Section 6.1 and Appendix C.4.
According to the experimental results in Table~\ref{tab:Hetro}, SLADE-Hetero demonstrates slightly improved performance compared to the original SLADE.
Nonetheless, SLADE's performance on actual dynamic heterogeneous graphs remains uncertain. As further research and datasets relevant to dynamic anomalous node detection in dynamic heterogeneous graphs emerge, we anticipate this could provide a promising direction for the future development of SLADE.
}

\begin{table}[H]
    \centering
    \caption{\label{tab:Hetro} AUC (in \%) in the detection of dynamic anomaly nodes with SLADE and SLADE-Hetero on dynamic bipartite graphs. }
    \setlength{\tabcolsep}{2.5pt}
    \small
    \scalebox{1.0}{
        
        \begin{tabular}{l|cc}
            \toprule
            Method & Wikipedia & Reddit   \\
            \midrule
            \midrule
                SLADE & 87.75 $\pm$ 0.68   & 72.19 $\pm$ 0.60     \\
                \tb{\method-Hetero}
                 &\bf{87.96 $\pm$ 0.41}  & \bf{72.65 $\pm$ 0.51}     \\
            \bottomrule
        \end{tabular}
}
    \vspace{-2.5mm}
\end{table}
